# Supplementary material for: Anomalous transport regime in non-Hermitian, Anderson-localizing hybrid systems
Source: arXiv:2206.05280 source file (2022-06-10)
Supplement: Supplementary file 1 [file Supplementary_information.pdf]

# Supplementary Information for

# Anomalous transport regime in non-Hermitian, Anderson-localizing hybrid systems

Himadri Sahoo[a,b], R Vijay[c], and Sushil Mujumdar[a]

[a] Nano-optics and Mesoscopic Optics Laboratory, Tata Institute of Fundamental Research, 1 Homi Bhabha Road, Mumbai 400005, India;
[b]Nanophotonics Laboratory, Department of Physics and Nanotechnology, SRM Institute of Science and Technology, Kattankulathur, Tamil Nadu 603203, India;
[c]Department of Condensed Matter Physics and Materials Science, Tata Institute of Fundamental Research, 1 Homi Bhabha Road, Mumbai 400005, India

*Corresponding author: Sushil Mujumdar
Email: mujumdar@tifr.res.in

## This file includes:

- **Section S1:** Band formation in SSPP structures
- **Section S2:** Concept of hybridization and regime of hybridization in Spoof Surface Plasmon Polariton (SSPP) structures
- **Section S3:** Frequency pinning at bandedge for highly disordered configurations
- **Section S4:** Eigenmodes corresponding to phase jumps at anomalous transport regime(ATR)
- **Section S5:** Measured probability distribution of intensity in localized and anomalous transport regime(ATR)
- **Section S6:** Necklace state confirmation through eigenmodes, simulated and experimental transmission

## Section: S1

## Band formation in SSPP structures:

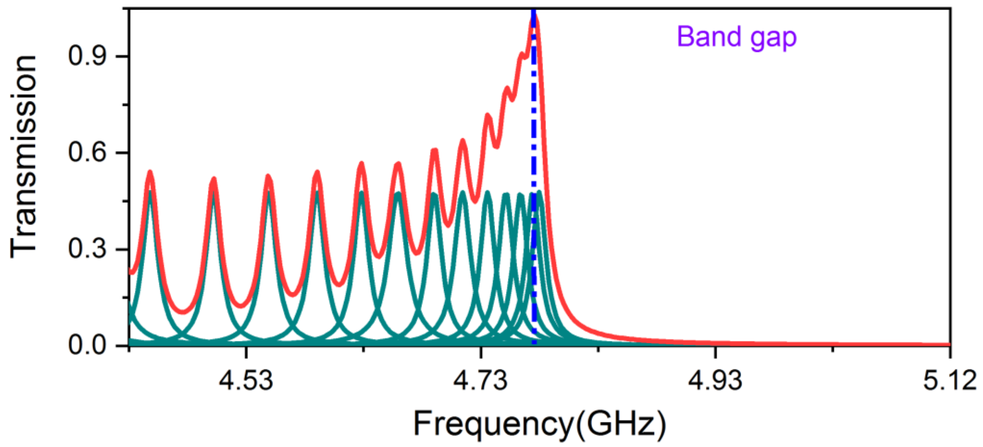


**Figure S1:** Lorentzians(dark cyan curves) corresponding to the eigenmodes existing in a periodic system. The bandedge appears at 4.77GHz(blue dashed line). Beyond the bandedge, no modes exist and this region constitutes the band gap. The width of the lorentzians decreases as they approach the bandedge. Red solid curve marks the corresponds the transmission.

In the plot for transmission vs frequency for the periodic system, the red solid curve represents the transmission and the dark cyan lorentzians indicate individual modes in the system. The blue dashed line represents the bandedge. For periodic system, the mode separation decreases as the modes approach the bandedge at 4.77 GHz. The band gap is devoid of modes.

## Section: S2

## Concept of hybridization and regime of hybridization in SSPP structures:

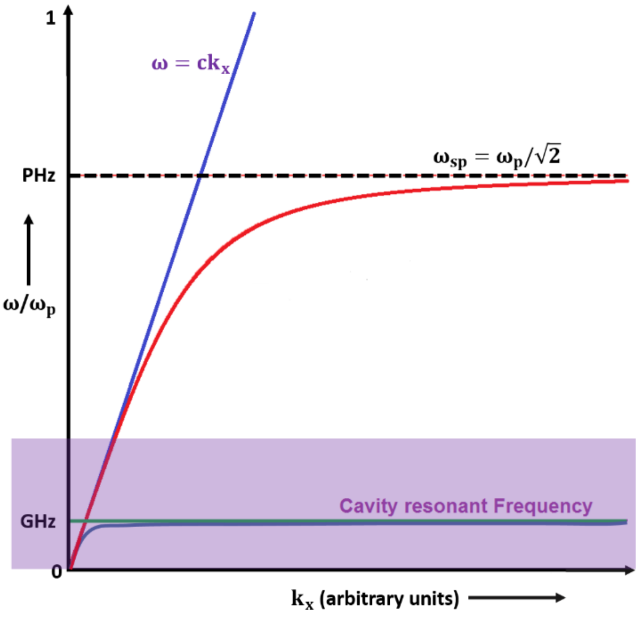


**Figure S2:** Dispersion plot for Surface plasmon polaritons (SPPs) existing at higher frequency range. The Spoof Surface Plasmon Polaritons (SSPPs) dispersion curve sets in at a lower range of frequency (GHz) as a consequence of hybridization of cavity resonant frequency with the polariton line.

If we consider the case of surface plasmon polaritons, the two interacting states are the plasma frequency due to electron oscillation and the photon frequency. This results in the avoided crossing of the two states thus forming the SPP dispersion curve or the polariton line. This avoided crossing is otherwise termed as hybridization. However, scientists were able to excite SPP like quasiparticles at the GHz and THz range by creating corrugations over the metal surface. They called these quasiparticles as Spoof or Designer Surface Plasmon Polaritons or SSPP in short. SSPPs are SPPs existing at lower frequency ranges.
SSPPs are formed due to the hybridization occurring as a result of interaction between the cavity resonant frequency of the corrugated structures and the plasmonic line. The inset shows the image of two unit cells of teeth like corrugated structure where the teeth height, h determines the cavity resonant frequency of our system which was determined to be at 5.35GHz.

## Section: S3

## Frequency pinning at bandedge for highly disordered configurations:

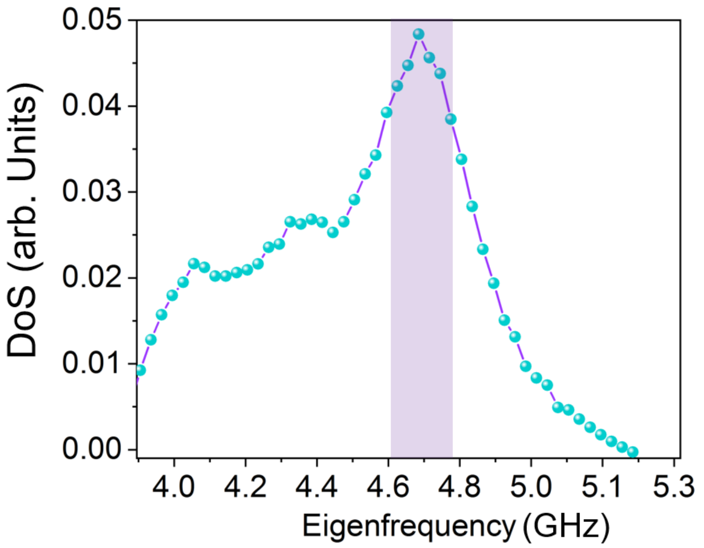


**Figure S3:** Probability of eigenfrequencies distribution plot for 56 highly disordered configs showing maximum eigenfrequencies exist around the bandedge (~4.77GHz). Modes migrate beyond the bandedge but never cross the hybridization frequency (5.35GHz) indicating frequency pinning in hybrid plasmonic systems.

In case of the disordered system, few modes migrate into the bandgap. The eigenvalues were obtained by eigensolver analysis of 56 highly disordered configurations. The above plot shows the probability of eigenfrequencies for these disordered configurations in which a frequency pinning of modes at the bandedge was observed. It has been previously shown in theory that in a hybrid plasmonic system, the modes under highest disorder does not cross the hybridization frequency. This holds true for our case as well, with no modes migrating beyond the hybridization frequency of 5.35GHz.

## Section: S4

## Eigenmodes corresponding to phase jumps at anomalous transport regime(ATR) :

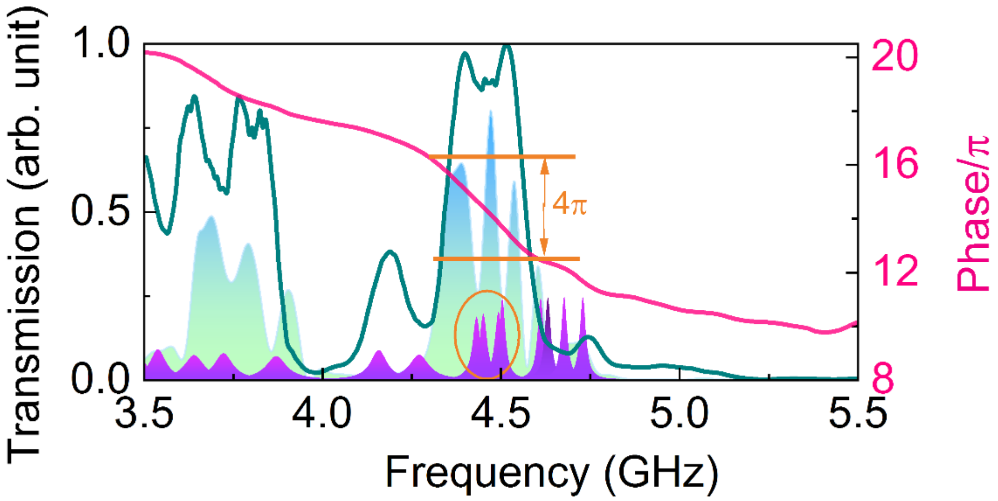


**Figure S4:** Component eigenvalues (shaded violet peaks) for the measured transmission spectrum as described in fig. 4. of the main manuscript reveal the participation of four resonances in the necklace as indicated by the orange ellipse.

A phase drop of nπ corresponding to the $n^{th}$ order necklace state occurs in the transmission. The corresponding eigenmodes contributing to the formation of necklace state is confirmed in simulation and indeed shows the presence of four eigenmodes overlapping spectrospatially that leads to an enhanced transmission observed in simulation as well as in experiment. Fig. S4 shows the component eigenvalues (shaded violet peaks) for the measured transmission spectrum of a highly disordered configuration that has a fourth order necklace state.

## Section: S5

## Measured probability distribution of intensity in localized and necklace regime:

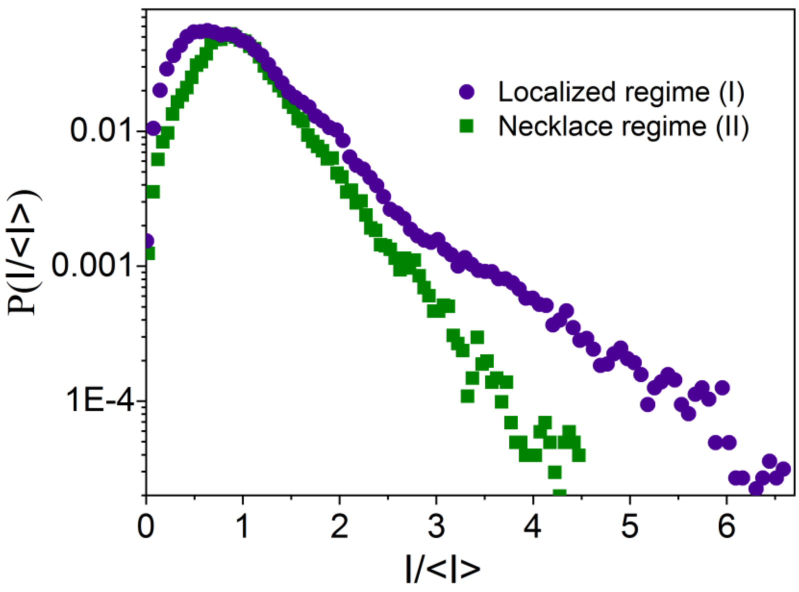


**Figure S5:** Measured probability distribution of normalized intensity, P(I/<I>), at two regimes: localized regime (violet dots) and necklace regime (green squares). I depicts the spatial intensity values of modes and <I> is their ensemble average.

Fig S5 shows the probability distribution of intensity, P (I/<I>) where I is the spatial mode intensity and <I> is their ensemble average intensity over 21 configurations at a high disorder strength. The violet and green scattered plots depict the localized and necklace regimes of transport respectively. In the localized case, the distribution shows large intensity fluctuations thereby significantly deviating from the Rayleigh distribution which is expected in the metallic (necklace) regime.

## Section: S6

## Necklace state confirmation through eigenmodes, simulated and experimental transmission:

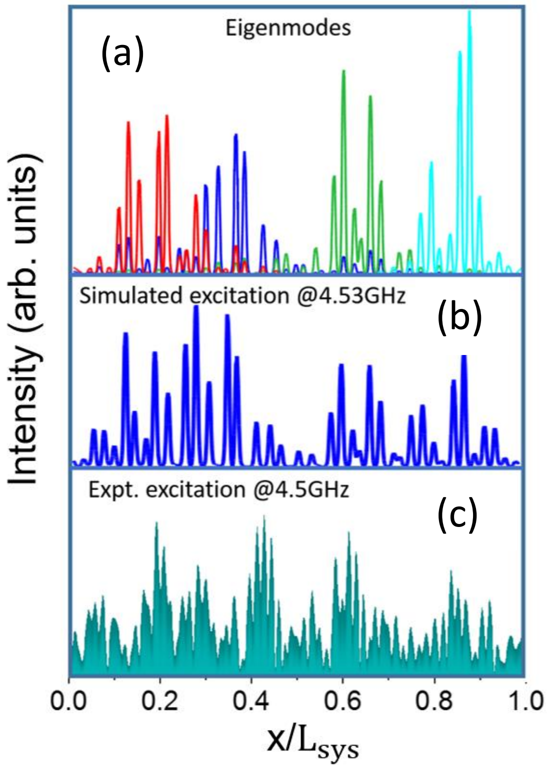


**Figure S5:** (a) Component eigenmodes corresponding to a fourth order necklace state existing for a highly disordered configuration, (b) shows the simulated 1-D spatial field profile of the excited necklace mode, (c) depicts the experimental excitation the necklace state encompassing the four eigenmodes.

Eigensolver analysis of the SSPP structure is shown in S5(a) that reveals four eigenfunctions (red, blue, green and cyan curves). The transmission in individual modes is minimal since they are weakly coupled to either end of the structure. However, a spectrospatial overlap between the modes, allows the SSPPs to hop through the localized states and undergo transmission. The corresponding simulated and measured intensity distribution is given by Fig. S5(b) (blue curve) and Fig. S5(c) (cyan curve) respectively when the system is excited at a frequency close to the bandedge frequency from the input (left) end of the array under strong disorder. Multiple peaks are seen in the intensity distributions. The intensity profile is seen to be a necklace of the four eigenmodes.
